# Supplementary material for: Matching the Clinical Reality: Accurate OCT-Based Diagnosis From Few Labels
Source: arXiv:2010.12316 source file (2020-10-23)
Supplement: Supplementary file 1 [file appendix_doc.tex]

\documentclass[runningheads]{llncs}

\usepackage{graphicx}
\usepackage{dirtytalk}
\usepackage{xcolor}
\usepackage{hyperref}
\usepackage{amsmath}
\usepackage{amssymb}
\usepackage{bbold}
\usepackage{booktabs} 
\usepackage[utf8]{inputenc}
\usepackage{pgfplots}
\usepackage{cite}
\usepackage{caption}
\usepackage{subcaption}

\begin{document}
\input{appendix}
\end{document}
